# Supplementary material for: Gaussian Splashing: Direct Volumetric Rendering Underwater
Source: arXiv:2411.19588 source file (2025-11-02)
Supplement: Supplementary file 1 [file back_algorithm.tex]

{
    \SetKwComment{Comment}{}{}
    \begin{algorithm}[h]
    \KwIn{$\lambda$}
    \KwData{$x$}
    \DontPrintSemicolon
 
  %  \Comment{// see text for convergence criteria}
   \caption{\TBD}%\label{alg:dpmeans}
    \end{algorithm}
    % \vspace*{1.0cm}
    }
